# Supplementary material for: Learning Simple Auctions
Source: arXiv:1604.03171 source file (2016-04-11)
Supplement: Supplementary file 1 [file appendix-multi.tex]

\section{Missing Proofs from the Multi-parameter section}\label{sec:appendix-multi}
\subsection{Multiple Additive Buyers}
\begin{prevproof}{Lemma}{lem:restricted}
  We first show these mechanisms are $\beta^i$-restricted. Since
  $\bv_i(\k) > 0$ only if $\v_i(\k) > \beta^i_\k$ neither $\bpi{i}(\beta^i)$ nor
  $\bpi{i}(\beta^i)$ will sell item $\k$ to $\bv_i$ unless $v_i(\k) > \beta^i_\k$,
  thus both are $\beta^i_\k$-restricted.

  We now show that both $\bpi{i}(\beta^i)$ and $\bri{i}(\beta^i))$, run on
  $\bv_i$, are incentive compatible and individually rational. First,
  buyer $i$ always prefers to win item $\k$ if she wins it according
  to this mechanism, since
  $v_i(\k) \geq \bv_i(\k) \geq \bp(\beta^i)_{\k}$. Thus, the item
  pricing mechanism is IR. Furthermore, an additive buyer $i$ has no
  reason to misreport $\v_i$; decreasing $\v_i(\k)$ does not affect
  the price of $\k$ but might cause her to lose $\k$ when she
  previously won (which, as before, she weakly prefers to win); nor
  will she want to increase $\v_i(\k)$, as it won't change
  $\bpi{i}(\beta^i)_{\k}$ but might cause $\bv_i(\k)$ to increase and
  allow her to win when she didn't previously, but only when
  $\bv_i(\k) < v_i(\k) \leq \max_{i'\neq i}v_{i'}(\k)$, so her price
  for $\k$ will be at least as large as $v_i(\k)$. Thus, running
  $\bpi{i}(\beta^i)$ on $\bv_i$ is also incentive-compatible for $v_i$.
  An analogous argument can be made for $\bri{i}(\beta^i)$ to prove its
  individual rationality and incentive compatibility.
\end{prevproof}

\begin{prevproof}{Lemma}{lem:independent}
  By assumption
  $((v_1(1), \ldots, v_n(1)), \ldots, (v_1(k), \ldots, v_n(k)))
  \sim \F^1\times \ldots \times \F^k$.
  Thus, for any function $f : \R^n \to \R^n$,
  \[(f(v_1(1), \ldots, v_n(1)) , \ldots, f(v_1(k), \ldots,
  v_n(k)))\sim \F'^1\times \ldots \times \F'^k,\]
  since $f$ is applied separately on each random variable drawn
  independently from a product distribution. Then, taking
  $f(v_1(\k), \ldots v_n(\k))_i = \bv_i(\k) = \v_i(\k)\cdot
  \mathbb{I}\lbrack[v_i(\k) > \max_{i'\neq i}v_{i'}(\k)\rbrack$
  proves the claim.
\end{prevproof}

\begin{prevproof}{Lemma}{lem:item-increase}
  First, notice that for any $\k$, $\bv_i(\k) > 0$ only if
  $v_i(\k) > \beta^i_k$.This implies that
  $\bv_i(\k) \geq \pik{i}{\k} > 0$ only if $v_i(\k) >
  \beta^i_\k$.
  Thus, if $\bv_i$ buys $\k$ at $\pik{i}{\k}$, she will also buy $\k$ at
  $\max (\pik{i}{\k}, \beta^i_k)$.  Finally,
  $\bpi{i}(\beta^i)(\k) \geq \pik{i}{\k}$, so the revenue of selling $\k$ is
  only larger. Thus, $\k$ is sold to $\bv_i$ by $\bpi{i}(\beta^i)$
  whenever it is sold to $\bv_i$ by $\np_{i}$, and is sold for a weakly
  larger payment, and the claim follows.
\end{prevproof}

\begin{prevproof}{Lemma}{lem:bundle-increase}
  For the set of items $\k$ such that $\bv_i(\k) > 0$, we know that
  $v_i(\k) > \beta^i_\k$. Thus, in particular,
  $\sum_{\k : \bv_i(\k) > 0} \bv_i(\k) = \sum_{\k : \bv_i(\k) > 0}
  v_i(\k) > \sum_{\k : \bv_i(\k) > 0} \beta^i_{\k}.$
  Thus, if $\sum_{\k : \bv_i(\k) > 0} \bv_i(\k) \geq \nri{i}$, it is
  also the case that
  $\sum_{\k : \bv_i(\k) > 0} \bv_i(\k) \geq \max(\nr_i, \sum_{\k :
    \bv_i(\k) > 0} \beta^i_{\k})$,
  so the bundle is sold to $\bv_i$ by $\bri{i}(\beta^i)$ whenever it
  was sold to $\bv_i$ by $\nri{i}$. As in the item pricing case, the
  revenue when the bundle is sold is weakly larger, so the claim
  follows.
\end{prevproof}
